# Supplementary material for: Byzantine Consensus in Abstract MAC Layer
Source: arXiv:2311.03034 source file (2023-11-06)
Supplement: Supplementary file 1 [file appendix-old.tex]

\appendix

\section{Analysis of rounds $3$ and $4$}
\label{app:converge}

In the following section, we calculate the bounds on $F$ and $S$ for rounds $3$ and $4$ to confirm that the generalization matches the pattern occurring within these rounds.

%\section{Analysis of rounds $3$ and $4$}


We now treat $F_2 \cup S_2$ as the ``input'' of the system. That is, we now suppose the minimum fault-free input in the system is $\frac{1}{4}$, and the maximum fault-free input in the system is $1$ for the case that $F_2 \cup S_2 = [\frac{1}{4}, 1]$. And, in the case that $F_2 \cup S_2 = [0, \frac{3}{4}]$, we treat $0$ as the minimum fault-free input, and $\frac{3}{4}$ as the maximum fault-free input. 

We will consider the case where $F_2 \cup S_2 = [\frac{1}{4}, 1]$. (The case where $F_2 \cup S_2 = [0, \frac{3}{4}]$ is analogous.)

\begin{lemma}
\label{lemma:f3}
    $F_3 = F_2 \cup S_2 = [\frac{1}{4}, 1]$ 
\end{lemma}

\begin{proof}
    By Lemma \ref{lemma:range}, $\frac{1}{4}\in F_3$ and $1\in F_3$, and by Lemma \ref{lemma:f-r+1}, $F_3 = F_2 \cup S_2$.
    %\item $\frac{1}{4}$ is a possible state when a first mover receives at least $2f + 1$ $\frac{1}{4}$'s and at most $f$ non-$\frac{1}{4}$'s. Note that Byzantine node can send any value.

    %\item $1$ is a possible state when a first mover receives at least $2f + 1$ $1$'s and at most $f$ non-$1$'s. Note that Byzantine node can send any value.

    %\item A value in the range $[\frac{1}{4}, \frac{5}{8}]$ is a possible state when a first mover receives at least $2f$ $\frac{1}{4}$'s and $f$ $1$'s from fault-free nodes and one random value in $[\frac{1}{4}, 1]$ from a Byzantine node. If this Byzantine node sends a $1$, the state will be $\frac{5}{8}$. Otherwise, the state will be in $[\frac{1}{4}, \frac{5}{8})$.

    %\item A value in the range $[\frac{5}{8}, 1]$ is a possible state when a first mover receives at least $2f$ $1$'s and $f$ $\frac{1}{4}$'s from fault-free nodes and one random value in $[\frac{1}{4}, 1]$ from a Byzantine node. If this Byzantine node sends a $\frac{1}{4}$, the state will be $\frac{5}{8}$. Otherwise, the state will be in $(\frac{5}{8}, 1]$.

    %\lewis{Are the last two cases needed?} 
\end{proof}

If $F_3$ does not have $\frac{1}{4}$ and/ or $1$, i.e. that $F_3 = (\frac{1}{4}, 1), (\frac{1}{4}, 1]$, or $[\frac{1}{4}, 1)$, then we  define the minimum value in $F_3$ to be 
%$x^F_3$ 
the minimum value of $F_2 \cup S_2$, namely, $x_2$ and the maximum value in $F_3$ to be 
%$y^F_3$, 
the maximum value of $F_2 \cup S_2$, namely, $y_2$. So the range for $F_3$ can be rewritten as %$[x^F_3, y^F_3]$. 
$[x_2, y_2]$ Then, we know that $F_3$ can then also have states 
%$[x^F_3, y^F_3]$ 
$[x_2, y_2]$ by Lemma \ref{lemma:range}. 

%\begin{lemma}
%\label{lemma:s3}
%    $S_3$ is either $[\frac{1}{4}, \frac{5}{8}]$, $[\frac{5}{8}, 1]$, $[x^F_3, \frac{x^F_3 + 1}{2}]$ or $[\frac{\frac{1}{4} + y^F_3}{2}, y^F_3]$; where $1 > x^F_3, y^F_3 > \frac{1}{4}$. %, $\frac{1}{4} < y_3 < 1$. %\callie{The upper bound for $S_3$ in any scenario is $1$, and the lower bound for $S_3$ in any scenario is $\frac{1}{4}$.} \lewis{What is the upper bound for $x_3$ and lower bound for $y_3$?}
%\end{lemma}

\begin{lemma}
\label{lemma:s3}
    $S_3$ is either $[\frac{1}{4}, \frac{5}{8}]$, $[\frac{5}{8}, 1]$, $[x_2, \frac{x_2 + 1}{2}]$ or $[\frac{\frac{1}{4} + y_2}{2}, y_2]$; where $1 > x_2, y_2 > \frac{1}{4}$. %, $\frac{1}{4} < y_3 < 1$. %\callie{The upper bound for $S_3$ in any scenario is $1$, and the lower bound for $S_3$ in any scenario is $\frac{1}{4}$.} \lewis{What is the upper bound for $x_3$ and lower bound for $y_3$?}
\end{lemma}

%\begin{proof}
    %We can apply an extension of the logic in Lemma \ref{lemma:s-1}.

    %Extending Lemma \ref{lemma:s-1}, we see that $S_3$ can either be $[\frac{1}{4}, \frac{5}{8}]$ or $[\frac{5}{8}, 1]$.

    %We also need to consider three other cases: (i) $F_3 = (\frac{1}{4}, 1)$, (ii) $F_3 = (\frac{1}{4}, 1]$, and (iii) $F_3 = [\frac{1}{4}, 1)$. %since it is possible to have values in between this range within the system (we do not know that there are only $\frac{1}{4}$'s and $1$'s at the inputs).


    %\begin{itemize}
        %\item $F_3 = (\frac{1}{4}, 1]$: 

        %By Definition \ref{def:r*}, we define the minimum value in $F_3$ to be $x^F_3$, so the range for $F_3 = [x^F_3, 1]$. Then, we know that $F_3$ can then have states $[x^F_3, 1]$ by Lemma \ref{lemma:range}.

    %\begin{itemize}
    %    \item $x_3$ is a possible state when a first mover receives at least $2f + 1$ $x_3$'s and at most $f$ non-$x_3$'s. Note that Byzantine node can send any value.
    %    \item $1$ is a possible state when a first mover receives at least $2f + 1$ $1$'s and at most $f$ non-$1$'s. Note that Byzantine node can send any value.
    %\end{itemize}

        %\item $F_3 = [\frac{1}{4}, 1)$: 
        %By Definition \ref{def:r*}, the maximum value in $F_3$ is $y^F_3$, so the range for $F_3 = [\frac{1}{4}, y^F_3]$. Then, we know that $F_3$ can then have states $[\frac{1}{4}, y^F_3]$ by Lemma \ref{lemma:range}

    %\begin{itemize}
    %    \item $\frac{1}{4}$ is a possible state when a first mover receives at least $2f + 1$ $\frac{1}{4}$'s and at most $f$ non-$\frac{1}{4}$'s. Note that Byzantine node can send any value.
    %    \item $y_3$ is a possible state when a first mover receives at least $2f + 1$ $y_3$'s and at most $f$ non-$y_3$'s. Note that Byzantine node can send any value.
    %\end{itemize} 

    %So, $S_3$ can also be $[x_3, \frac{x_3 + 1}{2}]$ or $[\frac{\frac{1}{4} + y_3}{2}, y_3]$.

        %\item $F_3 = (\frac{1}{4}, 1)$: 

    %\begin{itemize}
    %    \item $x_3$ is a possible state when a first mover receives at least $2f + 1$ $x_3$'s and at most $f$ non-$x_3$'s. Note that Byzantine node can send any value.
    %    \item $y_3$ is a possible state when a first mover receives at least $2f + 1$ $y_3$'s and at most $f$ non-$y_3$'s. Note that Byzantine node can send any value.
    %\end{itemize}
    %\lewis{Since we're using the observations above again and again. Maybe write a lemma about it so you can direclty apply.}

    %So, by the logic of Lemma \ref{lemma:s-1}, we see that $S_3$ can be $[x^F_3, \frac{x^F_3+y^F_3}{2}]$ or $[\frac{x^F_3+y^F_3}{2}, y^F_3]$. We know that $x^F_3 > \frac{1}{4}, y^F_3 < 1$, so $[x^F_3, \frac{x^F_3+y^F_3}{2}] \subset [x^F_3, \frac{x^F_3 + 1}{2}]$, and $[\frac{x^F_3+y^F_3}{2}, y^F_3] \subset [\frac{\frac{1}{4} + y^F_3}{2}, y^F_3]$. %so these are tighter cases and will cause the range to shrink faster than in the cases where $\frac{1}{4}$ and $1$ are included.
    %\end{itemize}
    
    
    %\lewis{These don't hold. Say $x_3 = y_3 = 0.9$. The upper bound is $0.9 > 5/8$} \callie{I changed this part to what I have in the paragraph above now.}
    
%\end{proof}

\begin{proof}
    We can apply an extension of the logic in Lemma \ref{lemma:s-1}.

    Extending Lemma \ref{lemma:s-1}, we see that $S_3$ can either be $[\frac{1}{4}, \frac{5}{8}]$ or $[\frac{5}{8}, 1]$.

    We also need to consider three other cases: (i) $F_3 = (\frac{1}{4}, 1)$, (ii) $F_3 = (\frac{1}{4}, 1]$, and (iii) $F_3 = [\frac{1}{4}, 1)$. %since it is possible to have values in between this range within the system (we do not know that there are only $\frac{1}{4}$'s and $1$'s at the inputs).


    \begin{itemize}
        \item $F_3 = (\frac{1}{4}, 1]$: 

        We know the minimum value in $F_3$ can be $x_2$, so the range for $F_3 = [x_2, 1]$. Then, we know that $F_3$ can then have states $[x_2, 1]$ by Lemma \ref{lemma:range}.

    %\begin{itemize}
    %    \item $x_3$ is a possible state when a first mover receives at least $2f + 1$ $x_3$'s and at most $f$ non-$x_3$'s. Note that Byzantine node can send any value.
    %    \item $1$ is a possible state when a first mover receives at least $2f + 1$ $1$'s and at most $f$ non-$1$'s. Note that Byzantine node can send any value.
    %\end{itemize}

        \item $F_3 = [\frac{1}{4}, 1)$: 
        We know the maximum value in $F_3$ is $y_2$, so the range for $F_3 = [\frac{1}{4}, y_2]$. Then, we know that $F_3$ can then have states $[\frac{1}{4}, y_2]$ by Lemma \ref{lemma:range}.

    %\begin{itemize}
    %    \item $\frac{1}{4}$ is a possible state when a first mover receives at least $2f + 1$ $\frac{1}{4}$'s and at most $f$ non-$\frac{1}{4}$'s. Note that Byzantine node can send any value.
    %    \item $y_3$ is a possible state when a first mover receives at least $2f + 1$ $y_3$'s and at most $f$ non-$y_3$'s. Note that Byzantine node can send any value.
    %\end{itemize} 

    %So, $S_3$ can also be $[x_3, \frac{x_3 + 1}{2}]$ or $[\frac{\frac{1}{4} + y_3}{2}, y_3]$.

        \item $F_3 = (\frac{1}{4}, 1)$: Combining the two above cases, we see that $F_3$ can be $[x_2, y_2]$

    %\begin{itemize}
    %    \item $x_3$ is a possible state when a first mover receives at least $2f + 1$ $x_3$'s and at most $f$ non-$x_3$'s. Note that Byzantine node can send any value.
    %    \item $y_3$ is a possible state when a first mover receives at least $2f + 1$ $y_3$'s and at most $f$ non-$y_3$'s. Note that Byzantine node can send any value.
    %\end{itemize}
    %\lewis{Since we're using the observations above again and again. Maybe write a lemma about it so you can direclty apply.}

    So, by the logic of Lemma \ref{lemma:s-1}, we see that $S_3$ can be $[x_2, \frac{x_2+y_2}{2}]$ or $[\frac{x_2+y_2}{2}, y_2]$. We know that when $x_2 > \frac{1}{4}$ and $y_2 < 1$, we have $[x_2, \frac{x_2+y_2}{2}] \subset [x_2, \frac{x_2 + 1}{2}]$, and $[\frac{x_2+y_2}{2}, y_2] \subset [\frac{\frac{1}{4} + y_2}{2}, y_2]$. %so these are tighter cases and will cause the range to shrink faster than in the cases where $\frac{1}{4}$ and $1$ are included.
    \end{itemize}
 
    
    %\lewis{These don't hold. Say $x_3 = y_3 = 0.9$. The upper bound is $0.9 > 5/8$} \callie{I changed this part to what I have in the paragraph above now.}
    
\end{proof}

Note that the difference between the minimum and maximum values in $[x_2, \frac{x_2 + 1}{2}]$ and $[\frac{\frac{1}{4} + y_2}{2}, y_2]$ is smaller than that in $[\frac{1}{4}, \frac{5}{8}]$ (and $[\frac{5}{8}, 1]$). %\lewis{This is a great observation, but it shouldn't be inside the proof.}



\begin{lemma}
\label{lemma:f4-u-s4}
    $F_4 \cup S_4$ is either $[\frac{1}{4}, \frac{7}{16}]$, $[\frac{13}{16}, 1]$, $[x^S_3, \frac{3x^S_3 + 1}{4}]$, or $[\frac{\frac{1}{4} + 3y^S_3}{2}, y^S_3]$.
\end{lemma}

\begin{proof}
    We consider four cases: 
    
    %We can extend Lemma \ref{lemma:at-most-f-1} and its application in Lemma \ref{lemma:f2-u-s2} to determine the possible bounds for $F_4 \cup S_4$.

    %To obtain bounds for $F_2 \cup S_2$ from the knowledge of $S_1$, we observe that 
    
    %\begin{itemize}
    %    \item When the lower bound for $F_2 \cup S_2$ remains constant, the upper bound becomes the mean of the minimum and maximum values of $S_1$. Similarly,
    %    \item When the upper bound for $F_2 \cup S_2$ remains constant, the lower bound becomes the mean of the minimum and maximum values of $S_1$. 
    %    \item \lewis{What if the cases above are not true?} \callie{I think I expressed this poorly ... I am going to make a general lemma to use here & below which I will explain more precisely.}
    %\end{itemize}

    We can apply Lemma \ref{lemma:fr-u-sr} to $F_4 \cup S_4$ using the mean of $S_3$ to find that:

    \begin{itemize}
        \item [(1)] When $S_3 = [\frac{1}{4}, \frac{5}{8}]$, $F_4 \cup S_4 = [\frac{1}{4}, \frac{7}{16}]$.
        \item [(2)] When $S_3 = [\frac{5}{8}, 1]$, $F_4 \cup S_4 = [\frac{13}{16}, 1]$.
        \item [(3)] When $S_3 = [x^S_3, \frac{x^S_3 + 1}{2}]$, $F_4 \cup S_4 = [x^S_3, \frac{3x^S_3 + 1}{4}]$.
        \item [(4)] When $S_3 = [\frac{\frac{1}{4} + y^S_3}{2}, y^S_3]$, $F_4 \cup S_4 = [\frac{\frac{1}{4} + 3y^S_3}{4}, y^S_3]$.
    \end{itemize}
\end{proof}

We can observe that the range for $F_4 \cup S_4$ has shrunk by at least $\frac{1}{4}$ again: %\lewis{More elaboration on this.}

\begin{itemize}
    \item We can see that in case (1) above, from $F_2 \cup S_2$ to $F_4 \cup S_4$, the range shrinks by $\frac{1}{4}$ since the difference between the minimum and maximum values changes from $1 - \frac{1}{4} = \frac{3}{4}$ in $F_2 \cup S_2$ to $\frac{7}{16} - \frac{1}{4} = \frac{3}{16}$ in $F_4 \cup S_4$ ($\frac{3}{4} \cdot \frac{1}{4} = \frac{3}{16}$). 

    \item Similarly, in case (2) above, from $F_2 \cup S_2$ to $F_4 \cup S_4$, the range shrinks by $\frac{1}{4}$ since the difference between the minimum and maximum values changes from $\frac{3}{4} - 0 = \frac{3}{4}$ in $F_2 \cup S_2$ to $1 - \frac{13}{16} = \frac{3}{16}$ in $F_4 \cup S_4$ ($\frac{3}{4} \cdot \frac{1}{4} = \frac{3}{16}$). 

    %\item %We have shown that the third and fourth cases above have smaller ranges than the first and second cases, so these will have shrunk by greater than $\frac{1}{4}$ as well. \lewis{I think you only showed $S_3$, but not really about $F_4 \cup S_4$, right?} \callie{I think $F_4 \cup S_4$ would be correct because Lemma 9 defines what $F_4 \cup S_4$ can be depending on the range of $S_3$.} 
    %\lewis{You need to the following two paragraphs to make the argument complete. They're not directly implied by what you showed above. Make each of them a standalone bullet point}

    \item In case (3) above, from $F_2 \cup S_2$ to $F_4 \cup S_4$, the range shrinks by $> \frac{1}{4}$ since the difference between the minimum and maximum values changes from $1 - \frac{1}{4} = \frac{3}{4}$ in $F_2 \cup S_2$ to $\frac{3x^S_3 + 1}{4} - x^S_3 = \frac{1 - x^S_3}{4}$ in $F_4 \cup S_4$. We know $\min\{S_3\} \leq x^S_3 \leq \max\{S_3\}$, and that $\frac{1}{4} < x^S_3 < 1$. Therefore, $\frac{1 - x^S_3}{4} < \frac{1 - \frac{1}{4}}{4} = \frac{3}{16}$. So $\frac{3}{4} \cdot \frac{1}{4} > \frac{1 - x^S_3}{4}$. 

    \item In case (4) above, from $F_2 \cup S_2$ to $F_4 \cup S_4$, the range shrinks by $> \frac{1}{4}$ since the difference between the minimum and maximum values changes from $\frac{3}{4} - 0 = \frac{3}{4}$ in $F_2 \cup S_2$ to $y^S_3 - \frac{\frac{1}{4} + 3y^S_3}{4} = \frac{y^S_3 - \frac{1}{4}}{4}$ in $F_4 \cup S_4$. We know $\min\{S_3\} \leq y^S_3 \leq \max\{S_3\}$ and that $\frac{1}{4} < y^S_3 < 1$. Therefore, $\frac{y^S_3 - \frac{1}{4}}{4} < \frac{1 - \frac{1}{4}}{4} = \frac{3}{16}$. So, $\frac{3}{4} \cdot \frac{1}{4} > \frac{y^S_3 - \frac{1}{4}}{4}$.  
    
    Therefore, in every case, the range of values in round $F_4 \cup S_4$ will shrink by at least $\frac{1}{4}$ as compared to $F_2 \cup S_2$. 
\end{itemize}
